# Supplementary material for: Nature of optical excitations in the frustrated kagome compound Herbertsmithite
Source: arXiv:1711.11340 source file (2017-11-30)
Supplement: Supplementary file 1 [file Pustogow_Herbertsmithite_supplement.pdf]

### Supplemental Material:

# Nature of optical excitations in the frustrated kagome compound Herbertsmithite

A. Pustogow,[1] Y. Li,[2] I. Voloshenko,[1] P. Puphal,[3] C. Krellner,[3] I.I. Mazin,[4] M. Dressel,[1] and R. Valentí[2]

[1] *1. Physikalisches Institut, Universität Stuttgart, 70569 Stuttgart, Germany*

[2] *Institut für Theoretische Physik, Goethe-Universität Frankfurt, 60438 Frankfurt am Main, Germany*

[3] *Physikalisches Institut, Goethe-Universität Frankfurt, 60438 Frankfurt am Main, Germany*

[4] *Code 6393, Naval Research Laboratory, Washington, DC 20375, USA*

## OPTICAL SPECTROSCOPY

In Fig. S1 (a) we present the in-plane reflectivity of $ZnCu_3(OH)_6Cl_2$ measured from the far-infrared up to the ultraviolet (40 - 47600 $cm^{-1}$) at normal incidence. While at low frequencies a constant value was extrapolated towards $\omega = 0$, at high frequencies the reflectivity was extrapolated by x-ray atomic scattering functions according to D. Tanner [1]. Panel (b) shows the optical conductivity calculated from the extrapolated reflectivity using the Kramers-Kronig relations (blue). It is in good agreement with the ellipsometric measurement (Fig. 3 (b) of the main manuscript) conducted at various angles of incidence $(20°, 30°, 40°, 50°, 60°)$ where $n$ and $k$ were obtained by simultaneously fitting the amplitude and phase coefficients $\Psi$ and $\Delta$ [2]. Note, due to their small intensity, the *d*-*d* excitations are observed only in the transmission signal and not in the reflectivity, where the signal-noise ratio does not allow resolving such a weak absorption feature [3, 4]. The sharp peaks at low frequencies correspond to lattice phonons [5].

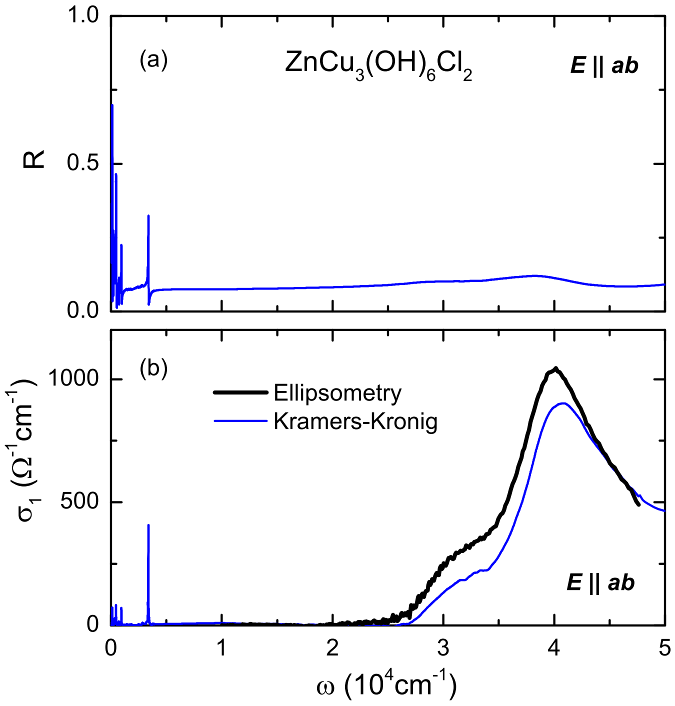


FIG. S1. (a) The broadband in-plane reflectivity of $ZnCu_3(OH)_6Cl_2$ measured at normal incidence. The sharp features at low energies correspond to lattice phonons [5]. Up to the visible range the reflectivity is flat and featureless indicating that absorption is very small inside the gap. (b) The optical conductivity was calculated from the reflectivity using the Kramers-Kronig relations (blue); it matches well with the result of our ellipsometric measurement (black).

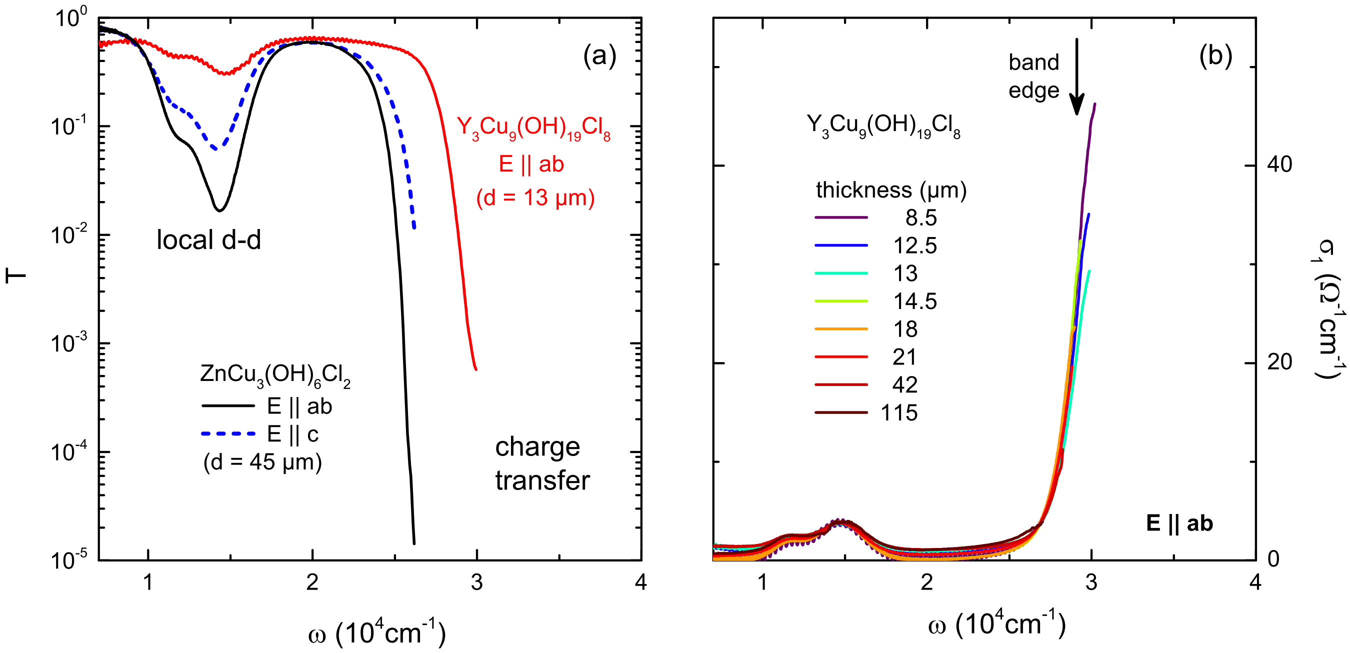


FIG. S2. (a) The transmission is plotted for a 45$\mu$m thick $ZnCu_3(OH)_6Cl_2$ sample ($E \parallel ab$ and $E \parallel c$) and a 13$\mu$m thick $Y_3Cu_9(OH)_{19}Cl_8$ crystal ($E \parallel ab$). The transmission could be determined reliably up to the onset of charge transfer transitions; at higher frequencies, the absorption is so large that the transmitted intensity below the detectable range. (b) The optical conductivity was directly calculated from reflectivity and transmission for $Y_3Cu_9(OH)_{19}Cl_8$ crystals of different thickness. The thinner the crystals (8.5 $\mu$m< $d$ < 115 $\mu$m), the larger the observed part of the band edge.

Fig. S2 (a) shows the transmission data of $ZnCu_3(OH)_6Cl_2$ and $Y_3Cu_9(OH)_{19}Cl_8$ used to determine $\sigma_1$ in Fig. 3 (a) of the main manuscript. Both the in- ($E \parallel ab$) and out-of-plane ($E \parallel c$) response could be measured for $ZnCu_3(OH)_6Cl_2$. Due to sample geometry – very thin, plate-like single crystals with the crystallographic $c$-direction oriented perpendicular to the surface – only the in-plane response could be determined for $Y_3Cu_9(OH)_{19}Cl_8$. On the other hand, the availability of differently sized samples allowed us to measure several single crystals of varying thickness to strengthen our results. As plotted in panel (b), the data collapse on top of each other for thickness variation of more than one order of magnitude, resulting in a precise mapping of the band edge.

Now we turn to the temperature dependence of the $d$-$d$ transitions, plotted in Fig. S3. Generally, transitions between octahedrally arranged Cu $d$-orbitals are dipole-forbidden. However, the selection rules are weakened if the center of symmetry is lost, either by structural deformation or vibronic coupling [3, 4, 6]. The latter effect is nothing but a time-dependent change of symmetry as the ligands are displaced with respect to the central Cu atom in the course of lattice vibrations. It is natural that such phononic contributions are relaxed upon cooling due to thermal activation. Moreover, the lattice contraction causes a blue-shift and corresponding spectral features become narrower. This is exactly what we observe in the temperature-dependent absorption of $Y_3Cu_9(OH)_{19}Cl_8$ shown in Fig. S3. The main characteristics, however, remain similar as in the high-temperature spectrum, which is consistent with the absence of a structural transition.

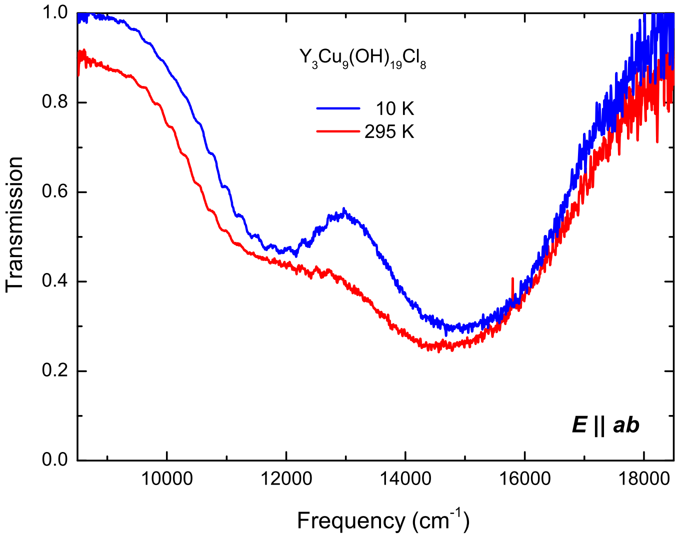


FIG. S3. The transmission of $Y_3Cu_9(OH)_{19}Cl_8$ was measured down to 10 K. As the temperature is reduced, the peaks exhibit a blue-shift and become slightly less intense, which is in line with a vibronic mechanism that activates the *d*-*d* transitions forbidden by the selection rules.

## STRUCTURAL ASPECTS

Table S1 lists the inter-atomic distances of $ZnCu_3(OH)_6Cl_2$ (Herbertsmithite) and $Y_3Cu_9(OH)_{19}Cl_8$ at room temperature [7, 8] following the notation of Fig. 2 (b) in the main paper. While the average Cu-O bond length is smaller by $\approx 0.4\%$, the Cu-Cl distance is slightly larger in the latter compound, which crystallizes in a Kapellasite-type structure [9] with the $Y^{+3}$ cations located within the Kagome layer. Thus, the $CuO_4Cl_2$ octahedra of $Y_3Cu_9(OH)_{19}Cl_8$ are a bit more stretched and, due to the inequivalent Cu sites, more distorted as compared to Herbertsmithite. On the other hand, the disparity between O-Cl distances is less pronounced than in $ZnCu_3(OH)_6Cl_2$ indicating that the $CuO_4$ plane is more parallel with respect to the equatorial plane perpendicular to the Cl-Cu-Cl axis (cf. Fig. 2 (b) of the main manuscript). Hence, the octahedra in $Y_3Cu_9(OH)_{19}Cl_8$ are closer to a rectangular shape.

TABLE S1. Inter-atomic nearest-neighbor distances within the $CuO_4Cl_2$ octahedra of $ZnCu_3(OH)_6Cl_2$ and $Y_3Cu_9(OH)_{19}Cl_8$ [7, 8]. For Herbertsmithite, the indices $i$ and $j$ take the values 1 or 2 with the constraint $i \neq j$. The Kapellasite-type compound $Y_3Cu_9(OH)_{19}Cl_8$ has two crystallographically inequivalent Cu sites implying more strongly distorted octahedra. The ratio between A and B sites is 1:2, where the latter one shows lower symmetry.

| Compound | $d_{CuO}$ | $d_{CuCl}$ | $d_{Oi-Oi}$ | $d_{Oi-Oj}$ | $d_{Oi-Cli}$ | $d_{Oi-Clj}$ |
|---|---|---|---|---|---|---|
| $ZnCu_3(OH)_6Cl_2$ | 1.983 | 2.777 | 2.612 | 2.981 | 3.195 | 3.617 |
| $Y_3Cu_9(OH)_{19}Cl_8$ (A) | 1.984\|1.987 | 2.761 | 2.936 | 2.673 | 3.193\|3.357 | 3.443\|3.599 |
| (B) | 1.960\|1.962\|1.980\|1.983 | 2.780\|2.823 | 2.811\|2.939 | 2.694\|2.701 | 3.193\|3.232\|3.357 | 3.508\|3.576\|3.583\|3.696 |

## THEORETICAL CALCULATIONS

### General considerations

In this Section we will discuss assumptions that implicitly or explicitly have been made during the calculations and which may adversely affect the agreement with the experiment.

One of the widely discussed deficiencies of the DFT in the LDA or GGA approximation is the fact that it routinely underestimates the band gaps. In conventional superconductors it is usually ascribed to the so-called "density derivative discontinuity" [10, 11], which manifests itself in the fact that the DFT potential can discontinuously change with an infinitesimally small change in the number of electrons. In strongly correlated materials the underestimation of the gap is related to Mott-Hubbard effects. It is often believed that correcting for this underestimation also corrects most problems of the calculated optical response within the density functional theory. In reality, however, the situation is more complex.

Indeed, most existing codes, including the one we used in this paper, employ the Random Phase Approximation (RPA). Formally, it can be written as

$$\varepsilon_{opt}(\omega) = 1 + V(q)\Pi(q,\omega)|_{q\to 0}, \tag{1}$$

where $V(q)$ is the Coulomb potential, and $\Pi(q,\omega)$ is the polarization operator. A more correct formula takes into account the local field effects, *i.e.*, rapid variation of the screening field, namely

$$\varepsilon_{opt}(\omega) = 1/[\varepsilon(\mathbf{G},\mathbf{G}',\omega)]^{-1}|_{\mathbf{G}=\mathbf{G}'=0}, \tag{2}$$

where the matrix $\varepsilon$ is written in the reciprocal lattice vector space, inverted, and then the first element is extracted from the inverse matrix. In the same notations, Eq. 1 can be written as

$$\varepsilon_{opt}(\omega) = \varepsilon(0,0,\omega). \tag{3}$$

Explicitly, it can be written as

$$\varepsilon(\mathbf{G},\mathbf{G}',\omega)^{-1} = \delta_{\mathbf{G},\mathbf{G}'} + V_C \cdot \Pi_0(q,\omega) \cdot [\delta_{\mathbf{G},\mathbf{G}'} - (V_C + I_{xc})\Pi]^{-1}, \tag{4}$$

where we have added the exchange-correlation local field to the Umklapp processes. Importantly, for $\mathbf{G},\mathbf{G}' \neq 0$ the Umklapp and the exchange-correlation local fields largely cancel each other. In DFT-LDA $I_{xc}(q)$ remains constant at small $q$, while $\Pi_0(q,0)$ vanishes as $q^2$, so that the net effect of the local field is small. At the same time, in an exact many-body theory or a reasonable approximation to it, such as the GW method, $I_{xc}$ diverges for small $q$ as $q^{-2}$ (reflecting the fact that the first exchange diagram in DFT includes two bubbles, and in Hartree-Fock only one). Thus, the exchange-correlation local field correction in the many-body approach is finite, and enhances the static dielectric function by a finite factor. In other words, compared to the many-body treatment, in DFT the RPA dielectric function is overestimated (since the gap is too small) and the local field enhancement is underestimated, and the two effects largely cancel each other. The corollary of this fact is that if a correction is applied to DFT calculations that enhances the gap, a similar correction should be applied to the RPA formula in form of a local field correction. As opposed to the GW method, LDA+$U$ or GGA+$U$ only do the former, but not the latter. Thus, while improving the *position* of the absorption peaks, LDA+$U$ or GGA+$U$ do a much worse job in calculating their intensity.

More detailed discussion of the physics outlined above can be found in Refs. [12, 13].

### Magnetic configuration

The conventional unit cell of Herbertsmithite includes three kagome Cu layers along the $c$ direction. There are three Cu in one layer for each unit cell. In order to make the antiferromagnetic (AFM) configuration, we constructed

a $2 \times 1 \times 1$ supercell. We used the same magnetic configuration for the three layers, and assumed six different AFM configurations for each layer using GGA+$U$. The lowest two energy configurations are chosen to calculate the optical conductivity. The resulting properties are similar. The one used in this paper is shown in Fig. S4.

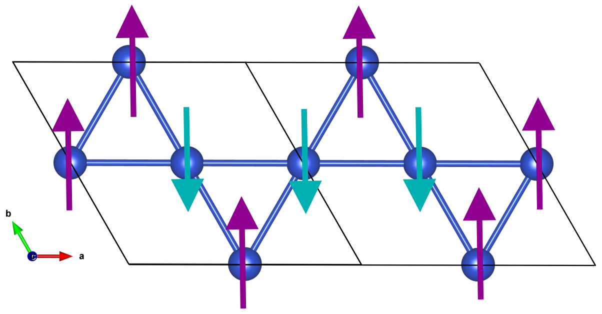


FIG. S4. Antiferromagnetic configuration of Cu for one of the layer used in GGA+$U$ calculations.

### The partial density of states and hopping parameters

The partial density of states with GGA for $ZnCu_3(OH)_6Cl_2$ are shown in Fig. S5. We consider 23 bands including Cu $d$, Cl $p$ and Zn $e_g$ orbitals; the corresponding on-site hopping parameters of Cu $d$ orbitals are shown in Table S2.

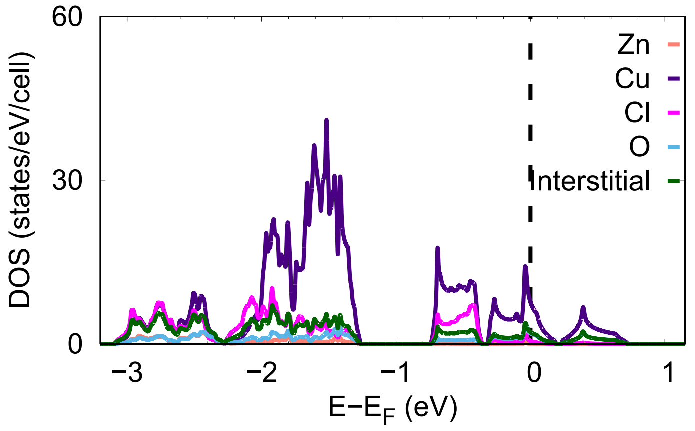


FIG. S5. Partial density of states for $ZnCu_3(OH)_6Cl_2$.

TABLE S2. Hopping parameters for the on-site terms (eV) in $ZnCu_3(OH)_6Cl_2$

| | $x^2-y^2$ | $z^2$ | $xz$ | $yz$ | $xy$ |
|---|---|---|---|---|---|
| $x^2-y^2$ | -0.160 | 0 | 0.006 | -0.006 | 0 |
| $z^2$ | 0 | -1.356 | -0.045 | -0.045 | -0.004 |
| $xz$ | 0.006 | -0.045 | -1.564 | 0.016 | 0.054 |
| $yz$ | -0.006 | -0.045 | 0.016 | -1.564 | 0.054 |
| $xy$ | 0 | -0.004 | 0.054 | 0.054 | -1.889 |

[1] D. B. Tanner, Phys. Rev. B **91**, 35123 (2015).
[2] H. Fujiwara, *Spectroscopic Ellipsometry* (John Wiley & Sons, Ltd, Chichester, UK, 2007).
[3] R. G. Burns, *Cambridge Topics in Mineral Physics and Chemistry*, 2nd ed. (Cambridge University Press, Cambridge, 1993).
[4] E. I. Solomon and A. B. P. Lever, *Inorganic electronic structure and spectroscopy* (Wiley & Sons, Inc., 1999) pp. 213–258.
[5] A. B. Sushkov, G. S. Jenkins, T.-H. Han, Y. S. Lee, and D. H. D, J. Phys.: Condens. Matter **29**, 95802 (2017).
[6] A. B. P. Lever, *Inorganic electronic spectroscopy* (Elsevier, Amsterdam, 1968).
[7] K. Mereiter, ICSD Collection Code 425835 (2013).
[8] P. Puphal, M. Bolte, D. Sheptyakov, A. Pustogow, K. Kliemt, M. Dressel, M. Baenitz, and C. Krellner, J. Mater. Chem. C **5**, 2629 (2017).
[9] R. H. Colman, C. Ritter, and A. S. Wills, Chem. Mat. **20**, 6897 (2008).
[10] J. P. Perdew and M. Levy, Phys. Rev. Lett. **51**, 1884 (1983).
[11] L. J. Sham and M. Schlüter, Phys. Rev. Lett. **51**, 1888 (1983).
[12] I. I. Mazin and R. E. Cohen, Ferroelectrics **194**, 263 (1997).
[13] I. I. Mazin, E. Maksimov, S. Rashkeev, and Y. Uspenskii, J. Exp. Theor. Phys. **63**, 637 (1986).
